# Supplementary material for: Differentially-Private "Draw and Discard" Machine Learning
Source: arXiv:1807.04369 source file (2018-10-10)
Supplement: Supplementary file 1 [file appendix_code.tex]

\subsubsection{R code to empirically estimate probability of having less than two pre-image candidates $t\gamma$ away (generates Figure~\ref{fig:k_vs_privacy} in Section~\ref{sec:multiple-preimages}).}\label{sec:code}
\bigskip

\scriptsize
\begin{verbatim}
library(rmutil)
library(RColorBrewer)

B <- function(gamma, epsilon) {
	2 * gamma / epsilon
}

V <- function(gamma, epsilon) {
	2 * B(gamma, epsilon)^2
}

L <- function(N, gamma, epsilon) {
	rlaplace(N, 0, B(gamma, epsilon))
}

Prob2N <- function(k, gamma, epsilon, N, frac) {
	ln <- L(N, gamma, epsilon)	
	inds <- matrix(sample(1:k, 2 * N, replace = TRUE), 2)

	mods <- rnorm(k, 0, sqrt(k/2 * V(gamma, epsilon)))
	two_neigh <- rep(0, N)
	for (i in 1:N) {
		mods[inds[1, i]] <- mods[inds[2, i]] + ln[i]
        neighbors <- sum(abs(mods[inds[1, i]] - mods) <= 
        	gamma * frac)
		two_neigh[i] <- neighbors < 3
	}
	mean(two_neigh)
}

gamma <- .001
epsilon <- 7
N <- 10000
colors <- rev(brewer.pal(n = 7, name = "Set2"))

ks <- seq(10, 100, 1)
probs <- matrix(0, 3, length(ks))
for (i in 1:length(ks)) {
	probs[1, i] <- mean(replicate(10, Prob2N(ks[i], gamma,
    	epsilon, N, frac = 1/10)))
	probs[2, i] <- mean(replicate(10, Prob2N(ks[i], gamma,
    	epsilon, N, frac = 1/5)))
	probs[3, i] <- mean(replicate(10, Prob2N(ks[i], gamma,
    	epsilon, N, frac = 1/2)))	
	cat(i, "\n")
}

plot(ks, probs[1, ], type = "l", ylim = c(0, .8),
	ylab = expression(paste("Prob(<2 pre-images within ", t,
    	gamma, ")")),
	xlab = "k", lwd = 2, col = colors[1], cex.lab = 1.2,
    	bty = "n")
lines(ks, probs[2, ], col = colors[2], lwd = 2)
lines(ks, probs[3, ], col = colors[3], lwd = 2)
legend("topright", legend = c("t=1/10", "t=1/5", "t=1/2"),
	fill = colors[1:3], bty = "n", border = colors[1:3],
    cex = 1.2)
\end{verbatim}
\normalsize
