# Supplementary material for: Differentially-Private "Draw and Discard" Machine Learning
Source: arXiv:1807.04369 source file (2018-10-10)
Supplement: Supplementary file 2 [file old_appendix.tex]

%\subsection{Privacy Proof Ideas}\label{sec:proof-ideas}
%Goals:
%\begin{itemize}
%\item Prove that privacy loss accumulates slower than as number of parameters times number of items submitted.
%\item Establish what role, if any, does the number of models $k$ play for privacy improvement.
%\item Establish what role, if any, does the ``forgetting'' property play for privacy improvement. Based on that, speculate what other models of forgetting one could use.
%\end{itemize}
%
%\subsubsection{Via Moments Accountant}
%\cite{mcmahanlanguage} and \cite{Abadi2016} both use moments accountant combined with sampling to get a tighter bound on their overall privacy loss than what one would obtain via an advanced composition theorem. 
%
%In our case, replacing the models at random is a variant of sampling. If we can analyze what sampling that gives us, we may also be able to apply moments accountant. Alternatively, if we can change the moments accountant computation to directly analyze our model sampling / replacement, we may be able to get a tighter bound.
%
%\subsubsection{Pre-image density}
%Perhaps related: What if noise added is not constant but a function of the number of models, number of points seen so far, etc?
%
%Perhaps related: \cite{bindschaedler2017plausible}
%
%\subsubsection{Via Hybrid Model}
%$k=1$ corresponds to trusted curator model, continual observation model
%$k=n$ corresponds to local model.
%
%We have something in-between. If we simply partitioned all users into one of the $k$ models, we'd have a trusted curator with each curator being entrusted with $\frac{n}{k}$ of the data. Since we have additional randomness -- curator assignment is random at each contribution, and we have random replacement, our privacy guarantees should be better! Can we first analyze strict partition without replacement; then add replacement?
%
%\cite{Prochlo} claim: $k=n$ stdev(noise) $\approx \sqrt{n}$; partition gives much benefit (see page 4, section 5.2).
%
%\subsubsection{Via a Relaxed Attacker Model and/or Privacy Definition}
%What if the realistic attacker is one that sees a random sample of the models that we have, rather than all of them?
%What if the realistic attacker is one that can inspect our $k$ models only after $1,000$ updates, rather than after every update? So a weaker model than streaming / continual observation.
%
%Average-case vs worst-case analysis?
%What is the connection to plausible deniability work, crowd-blending privacy, Renyi-DP, and smoothed sensitivity?
%
%In practice, the updates don't happen sequentially. By the time the server receives one update, many other models have changed.
%
%Can we say that recovering the input that happened 1,000 updates ago is more difficult than recovering the input that happened 1 update ago? Ultimately, it's addition where the order doesn't matter, so perhaps not? On the other hand, remember that each update happens also with noise, so even if all updates are zero, once one factors in the noise, the recovery is hard.
%
%\subsubsection{Privacy Impact of $k$}
%After $t$ steps, the probability that my data is still there is decreasing in $t$. So, on one hand, contributing my data helps derive a better gradient at some point, but long-term, the ``memory" of my data contribution is lost, as it was used on the gradient, not on the data itself.
%
%\begin{lemma}\label{lem:discard}
%As the number of updates goes to infinity, the probability that a particular contribution is present in any of the models goes to $\frac{1}{2}$.
%\end{lemma}
%


%\subsection{Via Model Over-Writing}
%\TODO{Vasyl: formalize the idea that the fact that we don't know whether the model was over-written or not gives a privacy boost.}
